# Supplementary material for: Validating Urban Scaling Laws through Mobile Phone Data: A Continental-Scale Analysis of Brazil's Largest Cities
Source: arXiv:2503.00550 source file (2025-03-01)
Supplement: Supplementary file 1 [file suplementarly-material.tex]

\documentclass[sn-apa]{sn-jnl}
%% 
%% Use one of the following options:
%% \documentclass[sn-apa]{sn-jnl}% APA Reference Style 
%% \documentclass[sn-chicago]{sn-jnl}% Chicago-based Humanities Reference Style
%% \documentclass[default]{sn-jnl}% Default
%% \documentclass[default,iicol]{sn-jnl}% Default with double column layout
%% \documentclass[sn-aps]{sn-jnl}% American Physical Society (APS) Reference Style
%% \documentclass[sn-vancouver,Numbered]{sn-jnl}% Vancouver Reference Style

%%%% Standard Packages
\usepackage{graphicx}%
\usepackage{xspace}%
\usepackage{multirow}%
\usepackage{amsmath,amssymb,amsfonts}%
\usepackage{amsthm}%
\usepackage{mathrsfs}%
\usepackage[title]{appendix}%
\usepackage{xcolor}%
\usepackage{textcomp}%
\usepackage{manyfoot}%
\usepackage{booktabs}%
\usepackage{algorithm}%
\usepackage{algorithmicx}%
\usepackage{algpseudocode}%
\usepackage{listings}%
\usepackage[normalem]{ulem} % For \sout{}

%%%% User-defined commands

%%%% Document begins
\begin{document}

\title[Supplementary Material]{Supplementary Material for the Paper:
{\it Validating Urban Scaling Laws through Mobile Phone Data: A Continental-Scale Analysis of Brazil's Largest Cities}}

%%=============================================================%%
%% Authors and affiliations
%%=============================================================%%
\author*[1]{\fnm{Ricardo} \sur{de S. Alencar}}\email{ricardo@lamce.coppe.ufrj.br}

\author[2]{\fnm{Fabiano} \sur{L. Ribeiro}}\email{fribeiro@ufla.br}
\equalcont{These authors contributed equally to this work.}

\author[3,4]{\fnm{Horacio} \sur{Samaniego}}\email{horacio@ecoinformatica.cl}
\equalcont{These authors contributed equally to this work.}

\author[5]{\fnm{Ronaldo} \sur{Menezes}}\email{r.menezes@exeter.ac.uk}
\equalcont{These authors contributed equally to this work.}

\author[1]{\fnm{Alexandre} \sur{G. Evsukoff}}\email{alexandre.evsukoff@coc.ufrj.br}
\equalcont{These authors contributed equally to this work.}

\affil[1]{\orgdiv{COPPE}, \orgname{Federal University of Rio de Janeiro}, \city{Rio de Janeiro}, \state{RJ}, \country{Brazil}}
\affil[2]{\orgdiv{Departamento de Física}, \orgname{Universidade Federal de Lavras}, \city{Lavras}, \state{MG}, \country{Brazil}}
\affil[3]{\orgdiv{Laboratorio de Ecoinformática, Instituto de Conservación, Biodiversidad y Territorio}, \orgname{Universidad Austral de Chile}, \city{Valdivia}, \country{Chile}}
\affil[4]{\orgdiv{Instituto de Sistemas Complejos de Valparaíso}, \city{Valparaíso}, \country{Chile}}
\affil[5]{\orgdiv{Department of Computer Science}, \orgname{University of Exeter}, \country{United Kingdom}}

\maketitle

\section{Overview}

This document provides additional methodological details, data descriptions, and robustness checks that complement the main text. By including supplementary figures, tables, and procedures, we aim to ensure that all relevant steps are reproducible and that our results are thoroughly supported.

\section{Details of the CDR Data, Selection Criteria, and Preprocessing}
\label{sec:CDR_data}

\subsection{Data Coverage and Descriptive Statistics}
Include a breakdown of how many users/calls per day exist in the dataset, aggregated by each of the 100 largest municipalities:
\begin{itemize}
    \item A table listing: City name, population, number of users, total calls, fraction of national total.
    \item A short description of the steps taken to remove incomplete or invalid records and the final dataset size.
\end{itemize}

\subsection{Antenna Coverage and Geospatial Visualization}
\begin{itemize}
    \item Provide maps of small, medium, and large municipalities to illustrate antenna placements and Voronoi polygons.
    \item Discuss potential biases in dense vs.\ sparse antenna coverage areas.
\end{itemize}

\subsection{User Residence Inference Details}
\begin{itemize}
    \item More extensive explanation of how nighttime calls are identified (e.g., 7~p.m.--6~a.m.\ on weekdays, all-day weekends).
    \item The fraction of users that do not meet the 50\% threshold and are excluded from the analysis.
    \item Any sensitivity checks on these thresholds.
\end{itemize}

\section{Additional Methodological Details}
\label{sec:additional_methods}

\subsection{Trip Detection Algorithm}
\begin{itemize}
    \item Detailed pseudocode for trip detection using consecutive calls, with justification for the 2\,km distance threshold and time constraints (30\,min--4\,h).
    \item Procedures for handling noise or GPS jitter.
\end{itemize}

\subsection{Sensitivity Analyses}
\begin{itemize}
    \item Demonstrate changes in the estimated exponents if different thresholds (e.g., 3\,km, 4\,km) are used.
    \item If the data span multiple months, show consistency across them.
\end{itemize}

\subsection{Degree Distribution Details}
\begin{itemize}
    \item Distribution plots (histograms, log-log, or CCDF) of $k_i$ for multiple cities.
    \item If fitting a functional form (e.g., log-normal), provide the fit parameters and quality metrics.
\end{itemize}

\section{Expanded Results and Robustness Checks}
\label{sec:expanded_results}

\subsection{City-by-City Breakdown of Main Variables}
Present a table with:
\begin{itemize}
    \item Population ($N$)
    \item Number of active users ($U$)
    \item Total calls, total trips (in the sample)
    \item GDP
    \item Number of antennas
\end{itemize}

\subsection{Alternative Regressions and Model Fits}
\begin{itemize}
    \item Use robust regression methods (e.g.\ RANSAC, Theil--Sen) to check for outlier effects.
    \item Possibly show bootstrapped confidence intervals for each exponent.
\end{itemize}

\subsection{Residual Analysis}
\begin{itemize}
    \item Include residual plots for key scaling regressions (GDP vs.\ population, total trips vs.\ population, etc.).
    \item Comment on whether patterns in residuals indicate any missing variables or non-linearities.
\end{itemize}

\section{Additional Context or Theoretical Extensions}

\subsection{Calls/Trips vs.\ Socioeconomic Factors}
\begin{itemize}
    \item If available, show correlations with city-level indicators like HDI, GINI, average household income.
    \item Discuss whether high-inequality or high-income cities deviate from the mean trend.
\end{itemize}

\subsection{Discussion of Potential Biases}
\begin{itemize}
    \item Revisit how a single-operator dataset can bias results, especially if certain cities are targeted by promotions or have strong competitor presence.
    \item Address the limitations of focusing on mostly prepaid plans if it might affect average or total degrees and trips.
\end{itemize}

\subsection{Exploratory Models}
\begin{itemize}
    \item If you tested alternative frameworks (gravity models, fractal city-size distributions) for cross-validation, mention them briefly.
\end{itemize}

\section{Data, Code, and Reproducibility}
\label{sec:reproducibility}

\subsection{Data Repository Information}
\begin{itemize}
    \item Provide a link to an online repository (e.g.\ Zenodo, OSF) where city-level aggregated data or scripts are hosted.
    \item Include a data dictionary or guide explaining columns and file structure.
\end{itemize}

\subsection{Code Snippets}
\begin{itemize}
    \item Examples of scripts for data cleaning, trip detection, degree calculation, and regression analysis.
    \item A link to a GitHub (or similar) repository, if journal policy permits.
\end{itemize}

\subsection{Ethical Considerations}
\begin{itemize}
    \item A summary of how privacy was protected (e.g., anonymization, no personal identifiers).
    \item Data-sharing agreements or institutional approvals, if relevant.
\end{itemize}

\section{Example Structure for Supplementary Material}

\begin{itemize}
    \item \textbf{Section S1: Extended Data Description and Preprocessing}
    \begin{itemize}
        \item Table S1.1: Raw data summary and cleaning steps
        \item Figure S1.1: Example antenna Voronoi diagrams
    \end{itemize}
    \item \textbf{Section S2: Residence Inference and User Selection}
    \begin{itemize}
        \item Figure S2.1: Distribution of night-time calls
        \item Table S2.1: Sensitivity of thresholds
    \end{itemize}
    \item \textbf{Section S3: Trip Detection Algorithm}
    \begin{itemize}
        \item Algorithm S3.1: Detailed pseudocode
        \item Table S3.1: Variation with distance/time thresholds
    \end{itemize}
    \item \textbf{Section S4: Degree Distributions}
    \begin{itemize}
        \item Figure S4.1: Example degree distributions
        \item Table S4.1: Log-normal or other fits
    \end{itemize}
    \item \textbf{Section S5: Robustness Checks and Residual Analysis}
    \begin{itemize}
        \item Figure S5.1: Residual plots
        \item Table S5.1: Alternative regression results
    \end{itemize}
    \item \textbf{Section S6: Additional Socioeconomic Correlations} (optional)
    \item \textbf{Section S7: Data Availability and Code}
    \begin{itemize}
        \item Links to repositories or data request procedures
    \end{itemize}
\end{itemize}

\section{Conclusion}

The above sections provide expanded detail on methods, data, and additional checks. By including these items, we aim to give a comprehensive view of our procedures and analyses, thereby enhancing the transparency and replicability of our results.

\end{document}
